# Supplementary material for: TexRel: a Green Family of Datasets for Emergent Communications on Relations
Source: arXiv:2105.12804 source file (2021-05-26)
Supplement: Supplementary file 1 [file 6_appendix.tex]

\appendix

\section*{Appendices}
